# Supplementary material for: InternVL-X: Advancing and Accelerating InternVL Series with Efficient Visual Token Compression
Source: arXiv:2503.21307 source file (2025-03-27)
Supplement: Supplementary file 1 [file experiments.tex]

\subsection{Experiments on other benchmarks}

% Due to the length limitation of the main paper, we only report the results on most benchmarks. In addition, we also evaluate our model on some other benchmarks, including AI2D \cite{ai2d}, ScienceQA \cite{scienceqa}, MME \cite{mme}, OKVQA \cite{okvqa}, HallusionBench \cite{hallusionbench} and RealWorldQA \cite{realworldqa}. As is shown in Tab. \ref{table7}, InternVL-X performs particularly well on natural science tasks, achieving the best results on ai2d and scienceqa, outperforming the previous best model LLaVA-NeXT by more than 5\% on average. On the MME benchmark, we also achieve results comparable to previous models. Finally, we achieve state-of-the-art results on the challenging HallB and RWQA tasks. These results demonstrate the comprehensiveness and reliability of our model.

Due to space constraints in the main paper, we primarily present our results on the most critical benchmarks. We have also undertaken extensive evaluations of our model on several additional benchmarks, including AI2D \cite{ai2d}, ScienceQA \cite{scienceqa}, MME \cite{mme}, OKVQA \cite{okvqa}, HallusionBench \cite{hallusionbench}, and RealWorldQA \cite{realworldqa}. As illustrated in Table \ref{table7}, our model, InternVL-X, exhibits exceptional performance in natural science-related tasks. It achieves top-notch results on the AI2D and ScienceQA benchmarks, surpassing the previous leading model, LLaVA-NeXT, by more than 5\% on average. Furthermore, on the MME benchmark, our model delivers performance that is on par with prior leading models. Notably, we have attained state-of-the-art outcomes on the particularly challenging HallusionBench (HallB) and RealWorldQA (RWQA) tasks. These superior results underscore the depth and reliability of our model’s capabilities, showcasing its robustness across a diverse array of challenging scenarios.

% \vspace{-2ex}

\begin{table}[h]
    \centering
    \resizebox{\linewidth}{!}
    {
        \begin{tabular}{@{}l@{\hskip 0.4em}@{\hskip 0.4em}l@{\hskip 0.4em}@{\hskip 0.4em}l@{\hskip 0.4em}@{\hskip 0.4em}l@{\hskip 0.4em}@{\hskip 0.4em}l@{\hskip 0.4em}@{\hskip 0.4em}l@{\hskip 0.4em}@{\hskip 0.4em}l@{\hskip 0.4em}@{\hskip 0.4em}l@{}}
            \toprule
                                Model                                     &AI2D    &SQA     &MME         &OKVQA    &HallB     &RWQA      \\
            \midrule
                                BLIP-2\cite{blip2}                     &-       &61.0    &-           &45.9     &-         &-        \\
                                LLaVA-1.5\cite{llava_1_5}               &-       &66.8    &1510/-      &-        &-         &-        \\
                                QwenVL\cite{qwenvl}                      &62.3    &67.1    &-           &58.6     &29.9      &-         \\
                                % \midrule
                                % InternVL-X                    &Internlm2-1.8B         &51.6   &60.5   &1348/279    &45.0    &30.3     &51.1  \\
                                InternVL-X                       &65.7   &73.8   &1462/348    &56.9    &37.3     &62.7    \\
                                \midrule
                                LLaVA-NeXT\cite{llavanext}             &66.6    &70.1    &1519/322    &51.4    &-         &-       \\
                                LLaVA-NeXT\cite{llavanext}            &60.8    &-       &1500/323    &-        &-         &54.4       \\
                                Monkey\cite{monkey}                       &62.6    &69.4    &1505/-      &61.3     &-         &-       \\
                                % \midrule
                                % InternVL-X-HD                 &Internlm2-1.8B         &57.3   &64.5   &1337/342    &46.2    &28.4     &54.1  \\
                                InternVL-X-HD                 &72.3   &73.9   &1499/369    &57.2    &38.2     &64.9    \\                            
    
            \bottomrule
            \end{tabular}
    }
    \caption{Comparison of InternVL-X and other MLLMs across 6 benchmarks.}
    \label{table7}
\end{table}

% \vspace{-2ex}

\subsection{Ablation study of multi-projector}

We conduct a comprehensive analysis of the impact of multi-projector on the model by assessing 3 parameters: the number of projectors $T$, the starting layer of projector insertion $w$, and the interval between projector insertion $i$. In our default configuration, we set $T=2$, $s=4$, and $i=4$. Our approach involves conducting ablation experiments by varying one parameter while keeping the others constant. We utilize the same 6 benchmarks from the main paper’s ablation experiment as our evaluation criteria. The results are illustrated in Fig. \ref{fig9}. In Fig. \ref{fig9_1}, we observe that adding more projectors consistently enhances model performance. When $T>=4$, the performance improvement tends to plateau and no longer shows significant gains. Fig. \ref{fig9_2} highlights that inserting projectors in shallow layers yields better results. Specifically, when $s<=4$, increasing $s$ leads to performance gains, but performance declines when $s > 4$. Fig. \ref{fig9_3} demonstrates similar phenomenon, the model performs best when $i=4$. Either reducing or increasing the interval negatively impacts the model’s effectiveness.

\begin{figure*}[!t]
    \setlength{\abovecaptionskip}{-2pt}
    \setlength{\belowcaptionskip}{2pt}
    \centering
    \begin{subfigure}{0.33\textwidth}
        \centering
        \includegraphics[height=1.2in]{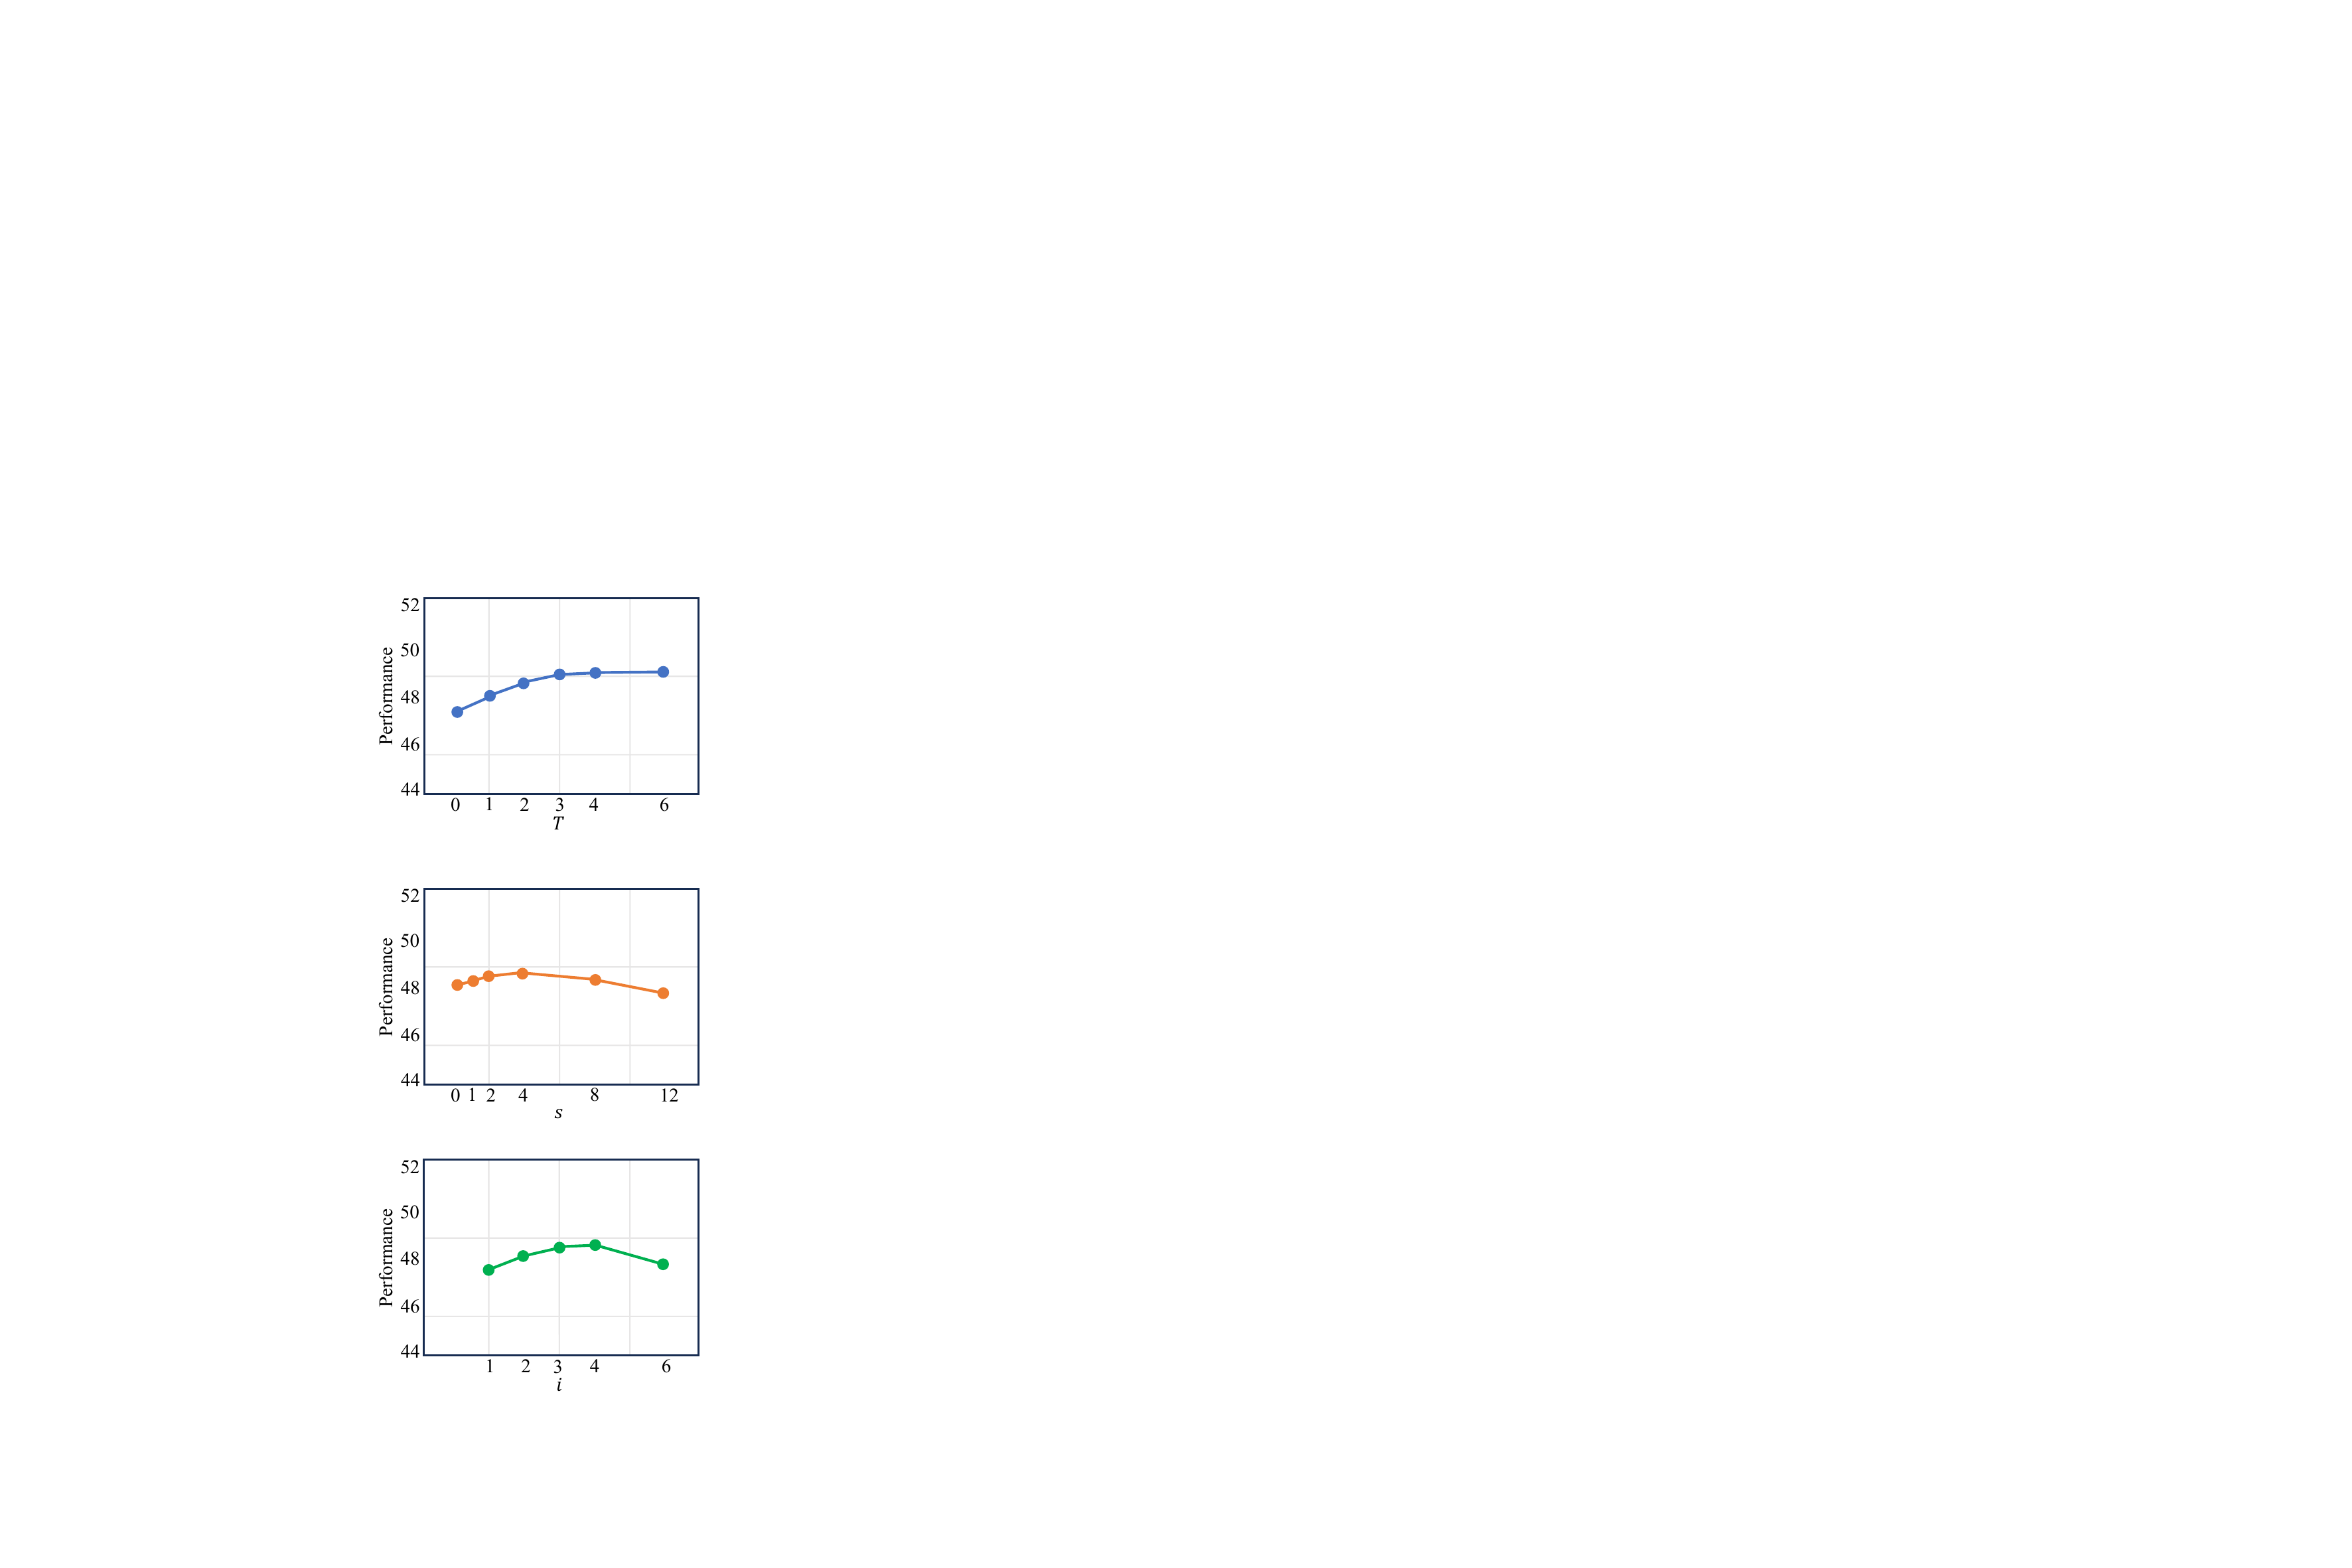}
        \caption{T layers}
        \label{fig9_1}
    \end{subfigure}
    \begin{subfigure}{0.33\textwidth}
        \centering
        \includegraphics[height=1.2in]{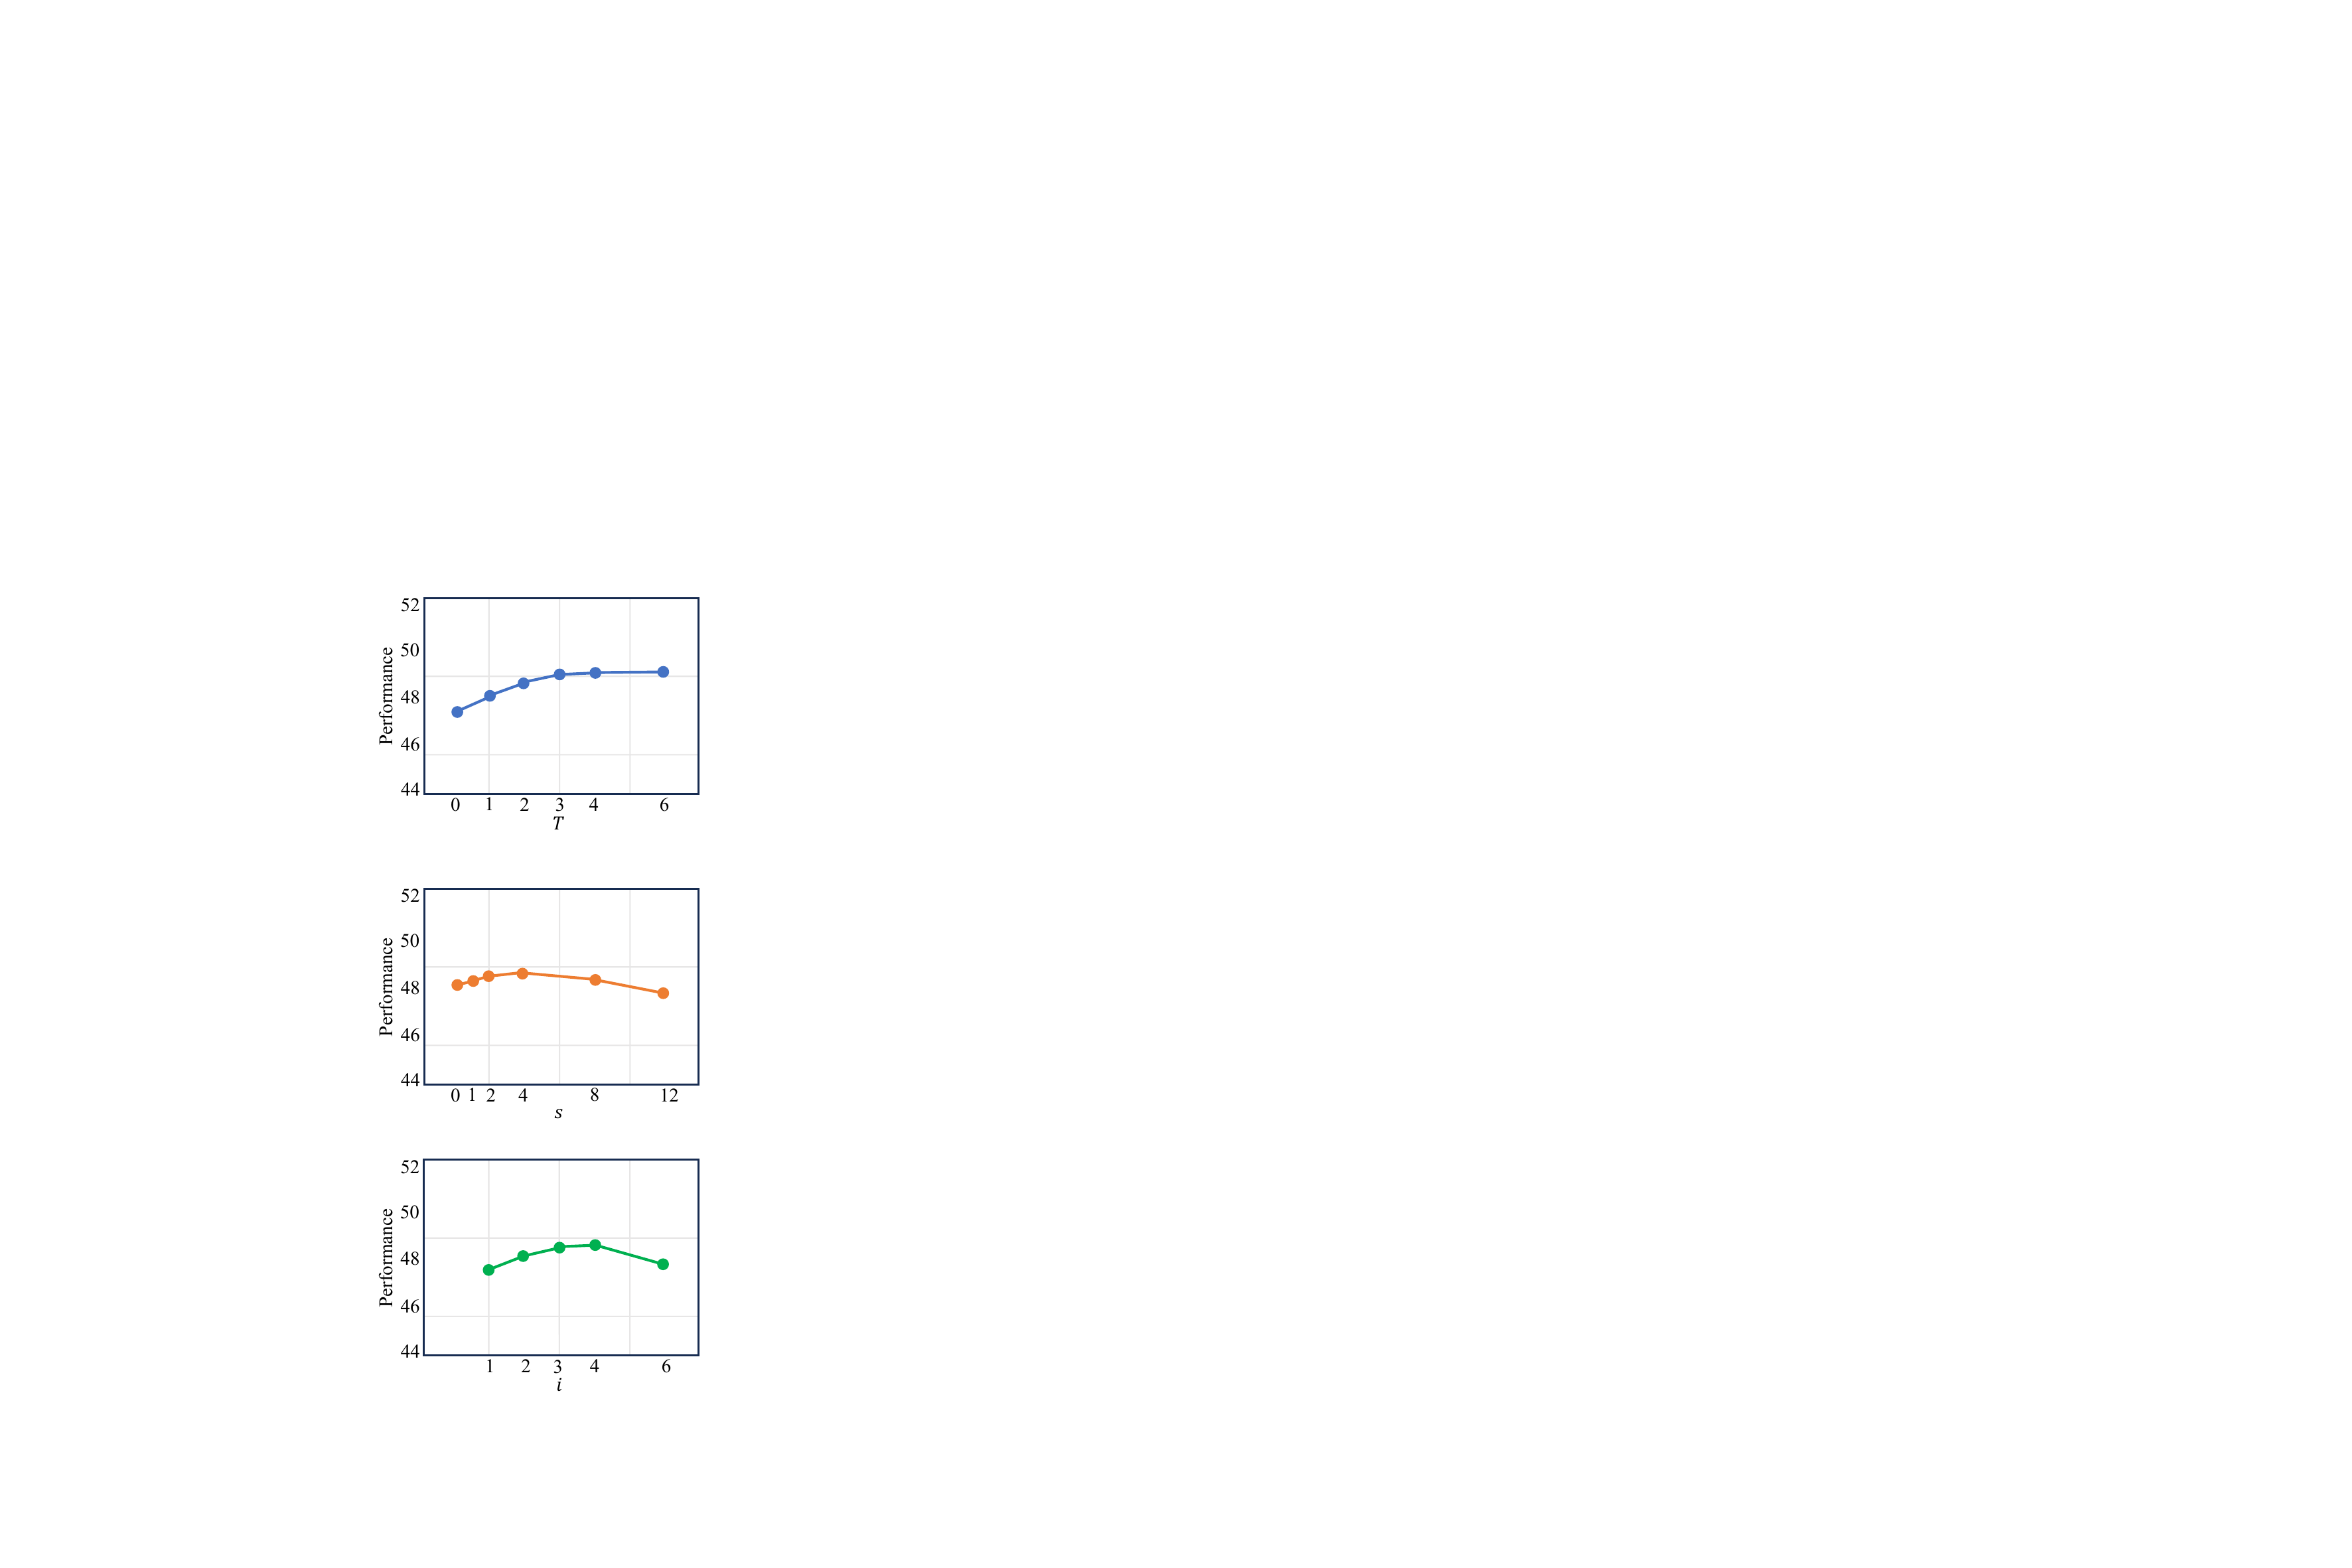}
        \caption{Starting layer}
        \label{fig9_2}
    \end{subfigure}
    \begin{subfigure}{0.33\textwidth}
        \centering
        \includegraphics[height=1.2in]{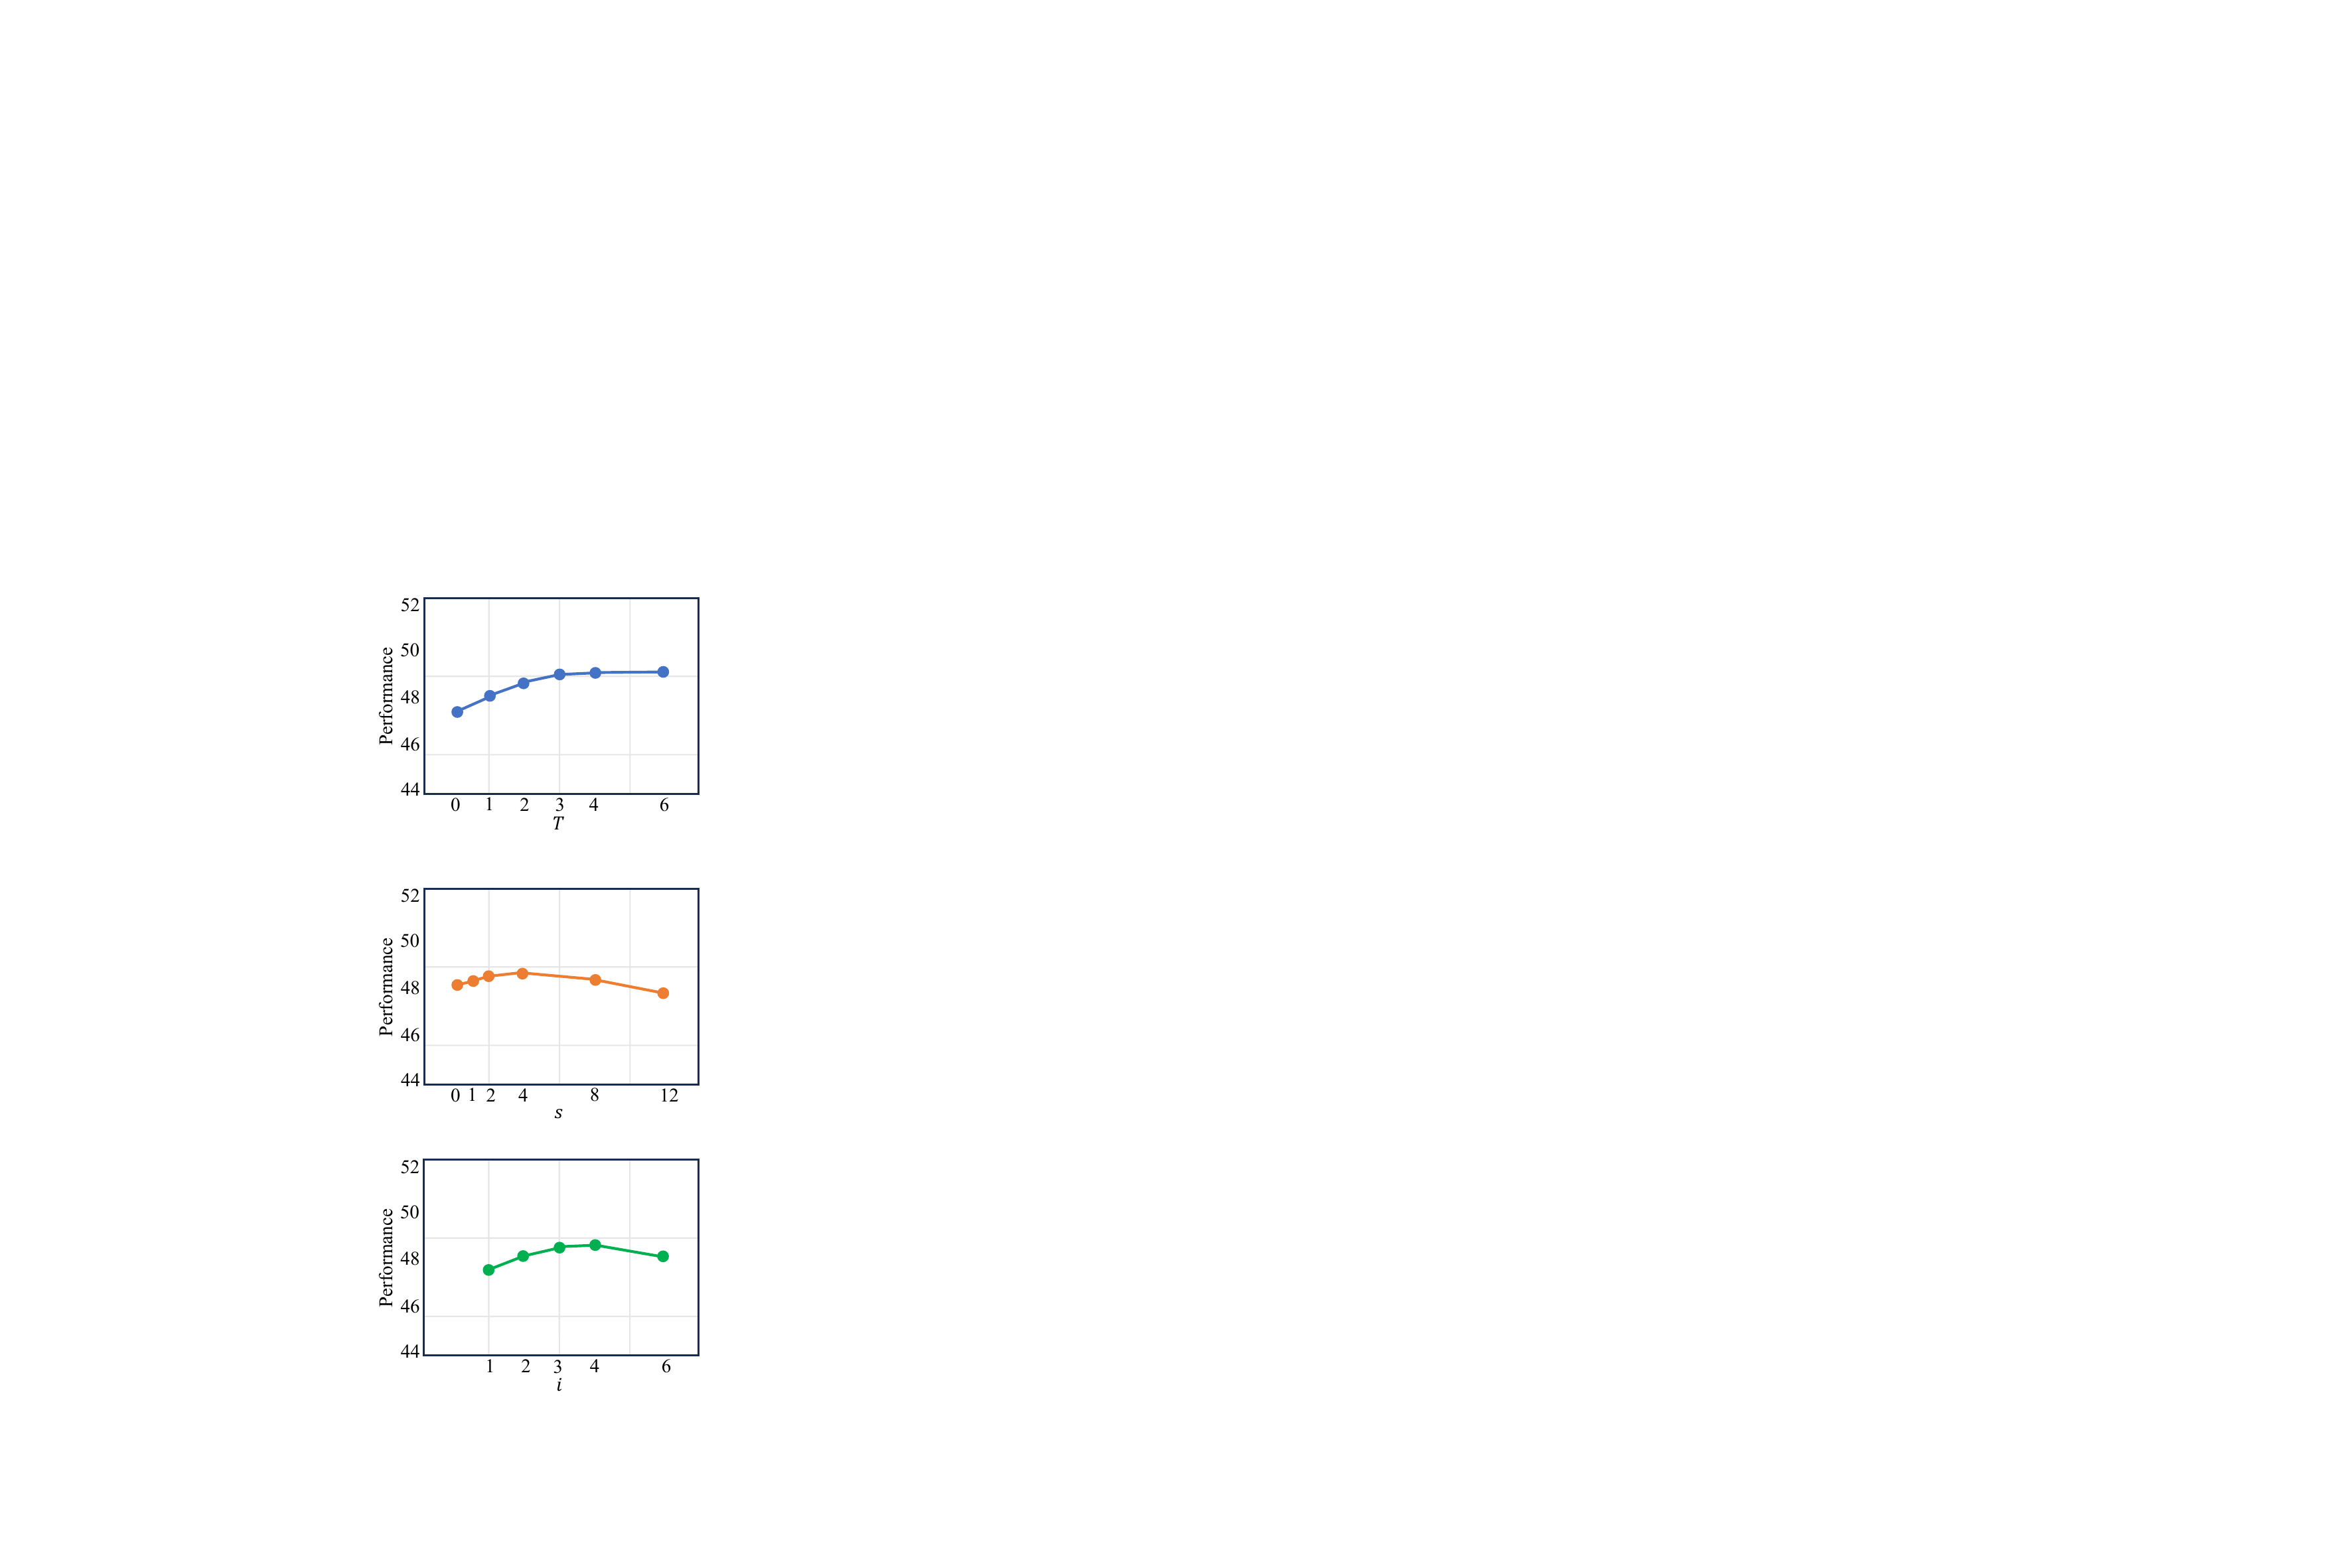}
        \caption{Interval}
        \label{fig9_3}
    \end{subfigure}
    \caption{Ablation study of multi-projector}
    \label{fig9}
  \end{figure*}

The multi-projector is not just a component of the LVTC framework, but can also be deployed as an independent module. Our idea draws inspiration from MOE \cite{moe} and Adapter \cite{adapter}. Each projector acts as an expert, contributing visual information related to various attributes or semantics to the middle layer of an LLM through an Adapter form. As multi-projector will increase the model parameters, we design it in a low-rank way, inspired by LORA \cite{lora}, to minimize this parameters. This multi-projector could be efficiently implemented using flash-attention with minimal resource usage. Consequently, it can be integrated with PVTC and RVTC, creating a model that offers dual benefits in terms of both performance and efficiency.
