# Supplementary material for: InternVL-X: Advancing and Accelerating InternVL Series with Efficient Visual Token Compression
Source: arXiv:2503.21307 source file (2025-03-27)
Supplement: Supplementary file 2 [file source_code.tex]

We provide the code for InternVL-X and VlmEvalkit. The model weights can be accessed at the following links: \href{https://huggingface.co/LLCC506/InternVL-X-2B}{InternVL-X-2B}, \href{https://huggingface.co/LLCC506/InternVL-X-8B}{InternVL-X-8B}, \href{https://huggingface.co/LLCC506/InternVL-X-2B-HD}{InternVL-X-2B-HD}, \href{https://huggingface.co/LLCC506/InternVL-X-8B-HD}{InternVL-X-8B-HD}. Since the flash-attention version of LVTC has not yet been implemented, the current code and weights only include implementations of PVTC and RVTC. Consequently, some metrics may differ from those reported in the main text.

To perform training, evaluation, and inference, please refer to the README\_InternVLX.md file in the repository.
