# Supplementary material for: InternVL-X: Advancing and Accelerating InternVL Series with Efficient Visual Token Compression
Source: arXiv:2503.21307 source file (2025-03-27)
Supplement: Supplementary file 3 [file visual_results.tex]

We evaluate InternVL-X against other models across a range of complex scenarios, including math, counting, visual perception, visual reasoning, charts, documents, and captioning, as illustrated in Figure \ref{fig10}. Compared to LLaVA-1.5, LLaVA-NeXT, and the InternVL2 (trained under the same conditions), InternVL-X provides more accurate answers and demonstrates superior performance across these diverse scenarios.

\begin{figure*}[h]
    \setlength{\abovecaptionskip}{2pt}
    \setlength{\belowcaptionskip}{-10pt}
    % \begin{center}
    \centering
    \includegraphics[width=6.75in]{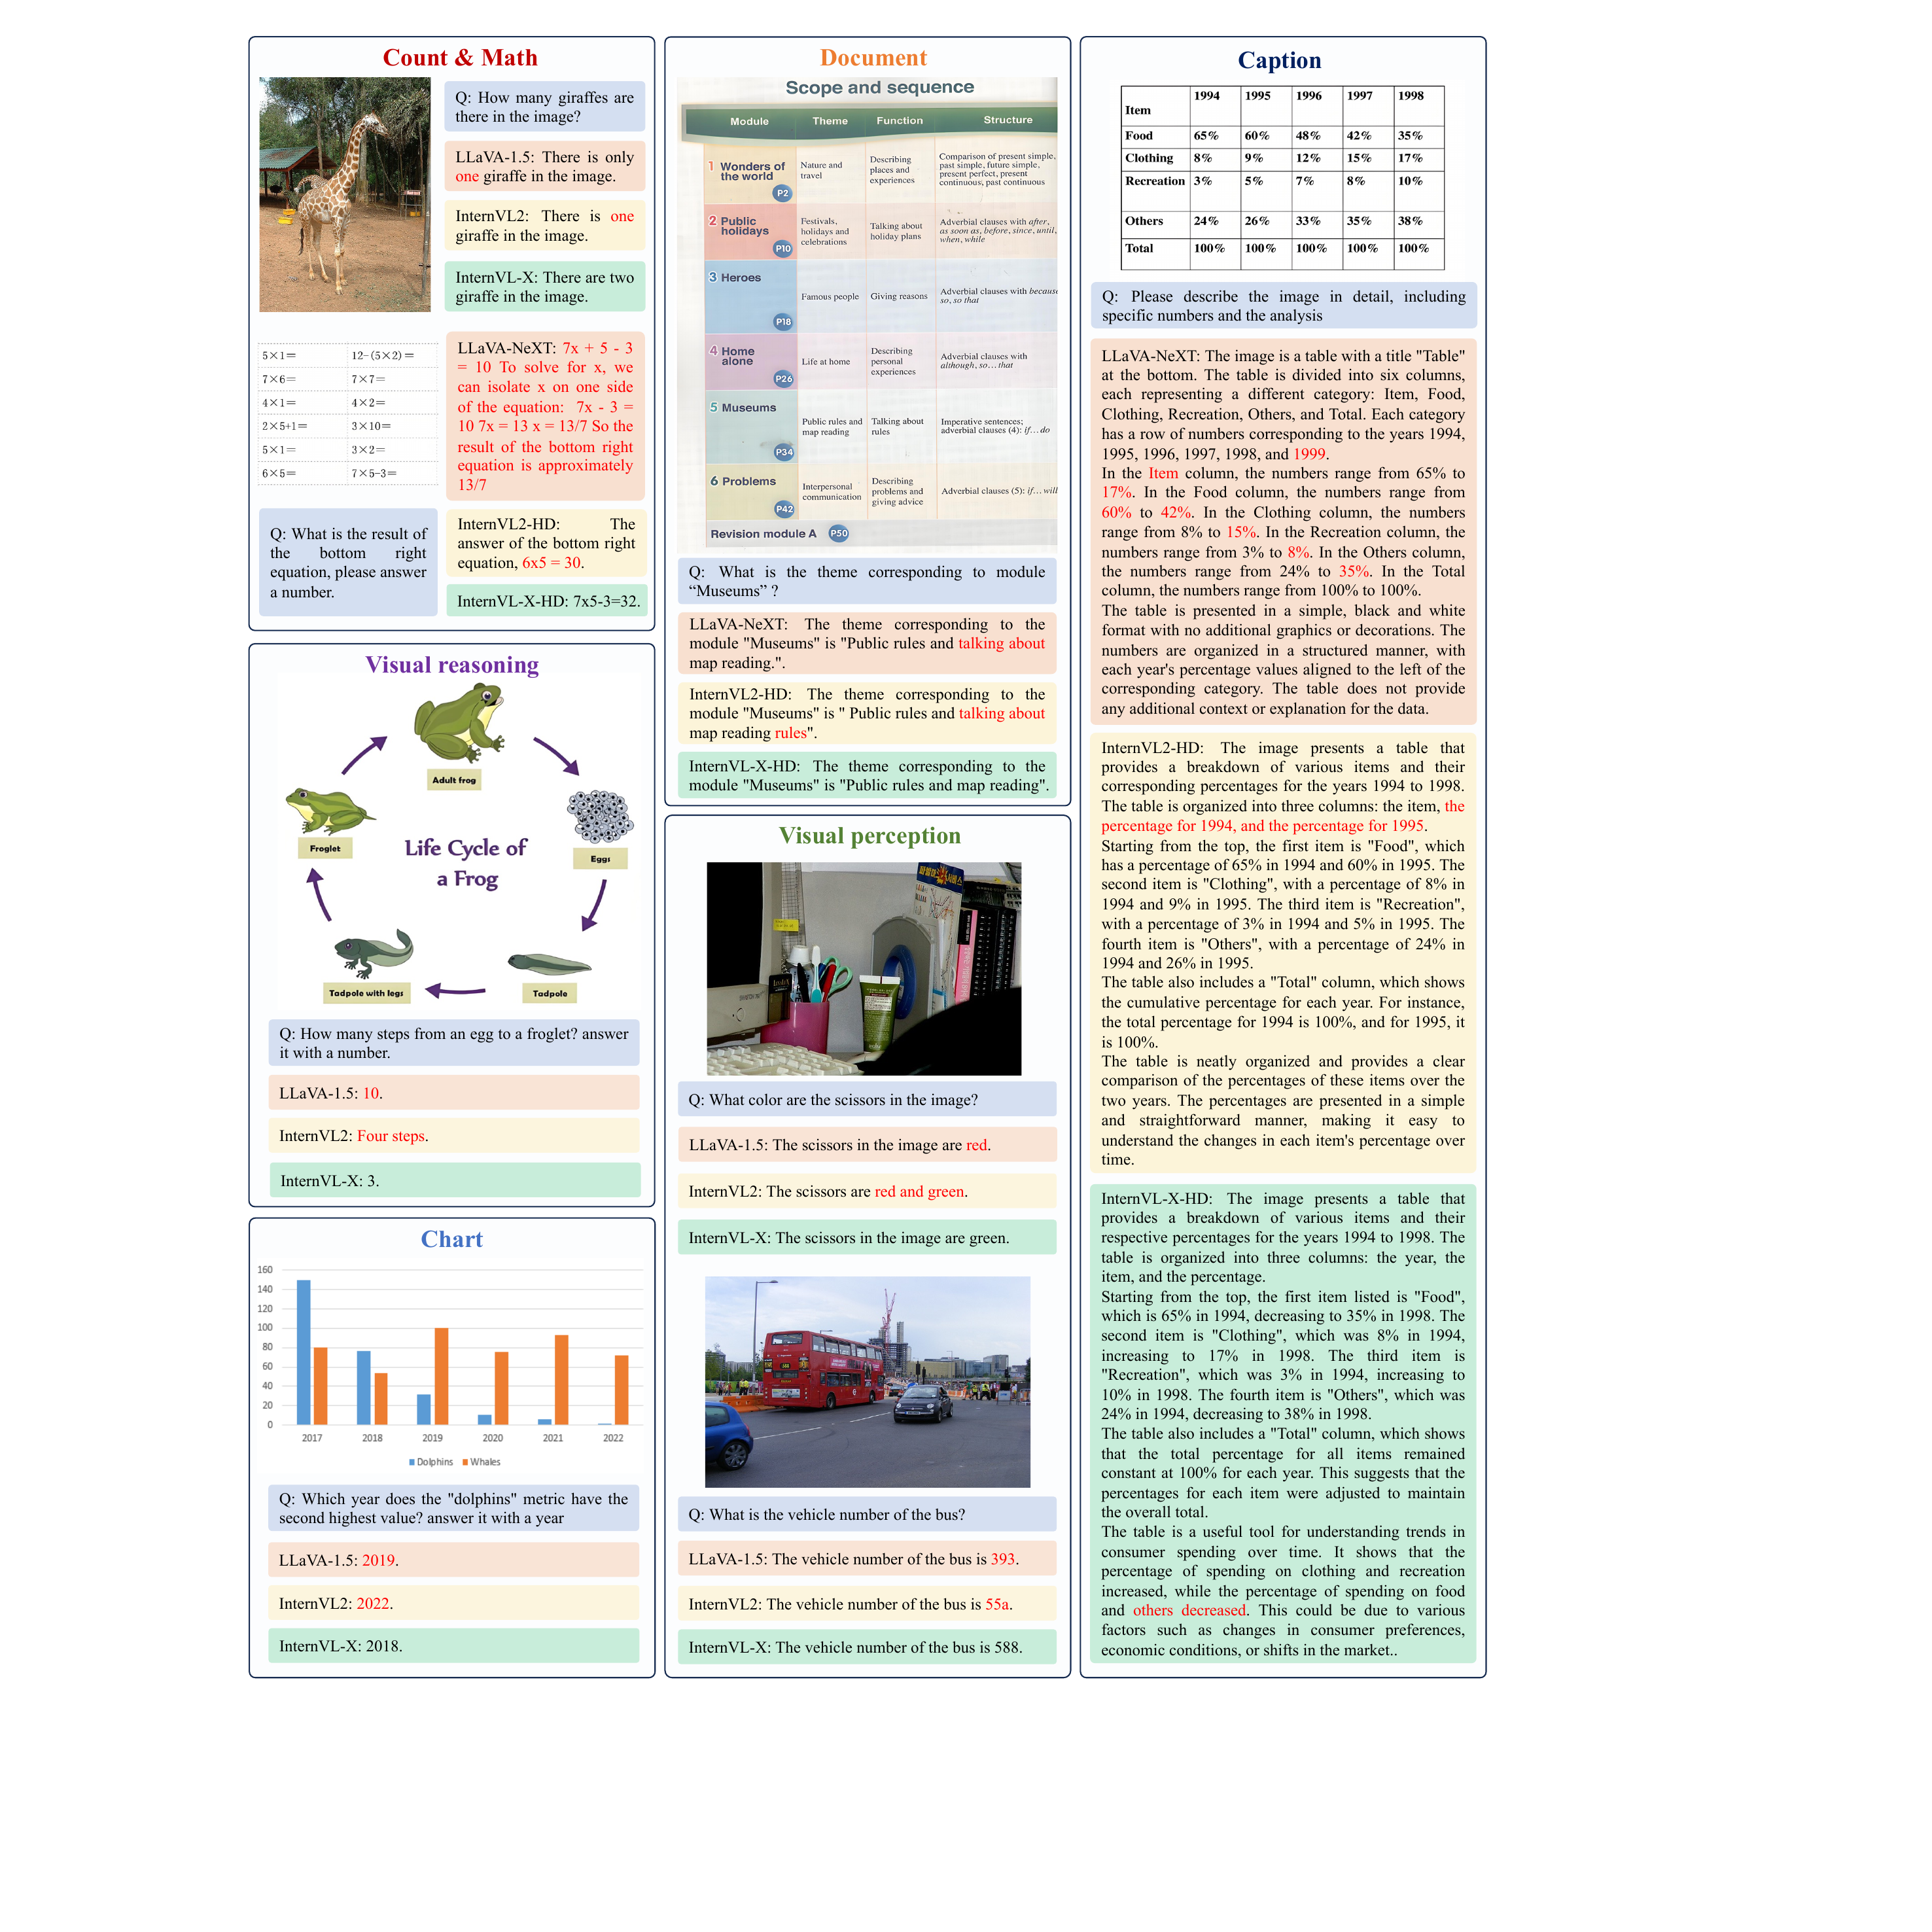}
    % \end{center}
    % \vspace{-2.5ex}
        \caption{Visual comparison of InternVL-X with other models. Red fonts represent incorrect answers.}
        \label{fig10}
\end{figure*}
